# Supplementary material for: Accelerating Moment Tensor Potentials through Post-Training Pruning
Source: arXiv:2510.19737 ancillary file (2025-10-22)
Supplement: Supplementary file 1 [file supporting_information.pdf]

# Supporting Information for Accelerating Moment Tensor Potentials through Post-Training Pruning

Zijian Meng,[*,†] Karim Zongo,[†] Matthew Thoms,[†] Ryan Grant,[‡] and Laurent Karim Béland[†]

†*Department of Mechanical and Materials Engineering, Queen's University, Kingston, ON Canada*

‡*Department of Electrical and Computer Engineering, Queen's University, Kingston, ON Canada*

E-mail: contact@richardzjm.com;17zjm1@queensu.ca

## MTP Implementation Details

The Moment Tensor Potential (MTP) is better described in the original paper by Shapeev.[1] We will focus on the practical implementation.

MTPs utilize linear regression on a basis set consisting of contractions of moment tensors. Each moment tensor, $M_{\nu,\mu}$ is characterized by a rank, $\nu$, and a $\mu$-indexed radial basis set. In the MLIP packages, each moment tensor has a level which is given by Eqn. 1.

$$\text{lev} M_{\nu,\mu} = 2 + 4\mu + \nu \tag{1}$$

Moment tensors can be contracted together. The level of these contractions is the sum of the levels of the constituent moment tensors. MTPs are specified by a level, and all scalar contractions whose level is less than or equal to an MTP's level are included in its basis set.

In their nickel-aluminum alloy parameterization, Wang *et al.* found improved performance by using Eqn. 2 instead.[2] This increases the number of radial basis sets.

$$\text{lev}M_{\nu,\mu} = 1 + 2\mu + \nu \tag{2}$$

In practice, it is inefficient to directly calculate these moment tensors and contract them because many intermediate values are repeated. Instead, a recursive style implementation reminiscent of dynamic programming is used where scalar contractions are decomposed into intermediate and basic values. This structure can be represented as a compute tree (directed acyclic graph). This compute tree is traversed in each neighborhood. Following Eqn. 1, MTP level 10's compute tree is shown in Fig. 1.

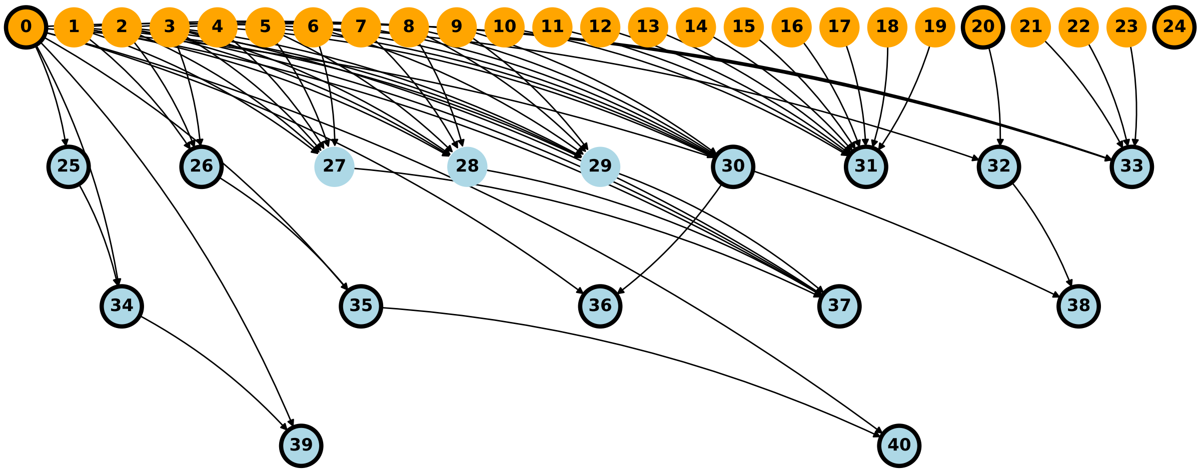


Figure 1: The compute tree of MTP level 10. Orange nodes are basic nodes, and outlined nodes are scalar contractions that form the MTP basis set.

There are $N_b$ basic nodes, each associated with a basic moment value specified by a precomputed tuple $(\mu, a, b, c)$, which is summed over all neighboring atoms of a central atom $i$, as defined in Eqn. 3.

$$\sum_j f_\mu(|\mathbf{r}_{ij}|, t_i, t_j) x_{ij}^a y_{ij}^b z_{ij}^c \tag{3}$$

Here, $|\mathbf{r}_{ij}|$ denotes the distance between atoms $i$ and $j$; $x_{ij}$, $y_{ij}$, and $z_{ij}$ are the components of the relative position vector of atom $j$ with respect to atom $i$; and $t$ indicates the atomic species. Notably, the cost of computing these $N_b$ basic nodes scales with the number of neighbors in the neighborhood. A precomputation step occurs before each neighbor is processed, where the powers of relative positions and the radial functions are cached.

The intermediate nodes are then constructed through $N_t$ sets of operations. The series of sets is predefined and, at runtime, each set accumulates the product of two previous nodes and a constant value. Since there are two previous nodes accessed in each set, edges are pruned two at a time, and the number of edges in a compute tree, $|E|$, is equal to twice the number of sets, $2N_t$.

The MTP may be linear relative to its basis set, but the radial parameters make the fitting non-linear. In the MLIP packages, the fitting uses a hybrid scheme. BFGS is used primarily, and a direction solution of the linear parameters is intermittently applied using Gaussian Elimination with pivoting.

# Accuracy Heuristic

We use the training loss, $\mathcal{L}(\boldsymbol{\theta})$, as described in the MLIP packages[3,4] as the accuracy objective function. Let the training set contain the configurations $\mathrm{cfg}_k$, for $k = 1, \ldots, K$, with known quantum-mechanical energies $E^{\mathrm{qm}}(\mathrm{cfg}_k)$, forces $\mathbf{f}_j^{\mathrm{qm}}(\mathrm{cfg}_k)$ for each atom $j = 1, \ldots, N_k$, and stress tensor $\boldsymbol{\sigma}^{\mathrm{qm}}(\mathrm{cfg}_k)$. The loss function is then given by Eqn. 4, where $E^{\mathrm{mtp}}$, $\mathbf{f}_j^{\mathrm{mtp}}$, and $\boldsymbol{\sigma}^{\mathrm{mtp}}$ are the MTP predictions for energy, forces, and stress, respectively; and $w_e$, $w_f$, and $w_s$ are their corresponding, user-defined weighting factors. There may be variations on this loss function used in practice.

$$\mathcal{L}(\boldsymbol{\theta}) = \sum_{k=1}^{K} \Bigg[ w_e \big(E^{\mathrm{mtp}}(\mathrm{cfg}_k;\boldsymbol{\theta}) - E^{\mathrm{qm}}(\mathrm{cfg}_k)\big)^2 + w_f \sum_{j=1}^{N_k} \sum_{\alpha=x,y,z} \big(\mathbf{f}^{\mathrm{mtp}}_{j,\alpha}(\mathrm{cfg}_k;\boldsymbol{\theta}) - \mathbf{f}^{\mathrm{qm}}_{j,\alpha}(\mathrm{cfg}_k)\big)^2 + w_s \sum_{\alpha,\beta=1}^{3} \big(\boldsymbol{\sigma}^{\mathrm{mtp}}_{\alpha\beta}(\mathrm{cfg}_k;\boldsymbol{\theta}) - \boldsymbol{\sigma}^{\mathrm{qm}}_{\alpha\beta}(\mathrm{cfg}_k)\big)^2 \Bigg] \tag{4}$$

Instead of handling $\mathcal{L}(\boldsymbol{\theta})$ non-linearly as is done in the MLIP packages, we freeze the radial parameters and only consider the linear parameters. Thus, the problem becomes that of solving an overdetermined linear system of equations using least squares. This is the matrix problem described by Thompson *et al.*[5] and shown in Eqn. 5, where $\mathbf{B}_i$ is $i$th basis function, and $\mathbf{r}_j$ is the relative position of the $j$th atom.

$$\begin{bmatrix} \vdots & \vdots \\ N_k & \sum_{i=1}^{N_k} \mathbf{B}_i(\mathrm{cfg}_k) \\ \vdots & \vdots \\ 0 & -\sum_{i=1}^{N_k} \frac{\partial \mathbf{B}_i(\mathrm{cfg}_k)}{\partial \mathbf{r}_{j,\alpha}} \\ \vdots & \vdots \\ 0 & -\sum_{j=1}^{N_k} \mathbf{r}_{j,\alpha} \sum_{i=1}^{N_k} \frac{\partial \mathbf{B}_i(\mathrm{cfg}_k)}{\partial \mathbf{r}_{j,\beta}} \\ \vdots & \vdots \end{bmatrix} \cdot \begin{bmatrix} \beta_0 \\ \boldsymbol{\beta} \end{bmatrix} = \begin{bmatrix} \vdots \\ E^{\mathrm{qm}}(\mathrm{cfg}_k) \\ \vdots \\ \mathbf{f}^{\mathrm{qm}}_{j,\alpha}(\mathrm{cfg}_k) \\ \vdots \\ \boldsymbol{\sigma}^{\mathrm{qm}}_{\alpha\beta}(\mathrm{cfg}_k) \\ \vdots \end{bmatrix} \tag{5}$$

This matrix formulation is of the type $\mathbf{X}\mathbf{b} = \mathbf{y}$ whose least squares solution can be determined by solving the normal equation, $(\mathbf{X}^\intercal\mathbf{X})\mathbf{b} = \mathbf{X}^\intercal\mathbf{y}$. To implement the weighting factors, a diagonal matrix $\mathbf{W}$ which contains the corresponding weights can be used with weighted least squares in Eqn. 6.

$$(\mathbf{X}^\intercal\mathbf{W}\mathbf{X})\mathbf{b} = \mathbf{X}^\intercal\mathbf{W}\mathbf{y} \tag{6}$$

For the indices of a subset of the basis functions, $A$, the weighted least squares would

solve $(\mathbf{X}_{AA}^\intercal \mathbf{W}_{AA} \mathbf{X}_{AA})\mathbf{b} = \mathbf{X}_{AA}^\intercal \mathbf{W}_{AA} \mathbf{y}_A$ where $_A$ represents a subvector, and $_{AA}$ represents a principal submatrix, formed by the indices of $A$.

Thompson *et al.* use QR factorization to solve Eqn. 5. This approach avoids explicitly forming the normal equations and consequently avoids squaring the condition number. For our heuristic evaluation, instability can be mitigated through Tikhonov regularization without significantly affecting the pruning. We chose a value of $\lambda$ that only ensures a bare minimum level of numerical stability ($\kappa \approx 10^{12}$). In the paper proposing the MTP,[1] Shapeev uses $\text{diag}(\mathbf{X}^\intercal \mathbf{X})$ as the penalization matrix instead of the identity matrix so that its scaling with respect to the database size and the scale of the basis functions is compatible with that of $(\mathbf{X}^\intercal \mathbf{X})$. However, we apply regularization solely to reduce the condition number and thus simply use the identity matrix.

Solving the normal equations is $\mathcal{O}(p^2 n + p^3)$ for a $n \times p$ $\mathbf{X}$ matrix. For an overdetermined system, $\mathbf{X}$ is a tall matrix: $n > p$. In the paper proposing the MTP,[1] Shapeev was briefly experimenting with $L_0$ regularization wherein he aimed to minimize the number of non-zero linear learnable coefficients, also using a similar genetic algorithm approach. As he noted, in exchange for explicitly forming $(\mathbf{X}^\intercal \mathbf{W} \mathbf{X})$, we can reformulate the weighted least squares for a subset of indices, $A$, as Eqn. 7.

$$(\mathbf{X}^\intercal \mathbf{W} \mathbf{X})_{AA} \mathbf{b} = (\mathbf{X}^\intercal \mathbf{W} \mathbf{y})_A \tag{7}$$

Both $(\mathbf{X}^\intercal \mathbf{W} \mathbf{X})$ and $(\mathbf{X}^\intercal \mathbf{W} \mathbf{y})$ can be precomputed, then efficiently masked off at runtime, reducing the time complexity to $\mathcal{O}(p^3)$. Moreover, being positive definite, a solver with a low constant term, like Cholesky Decomposition, can be applied effectively. Using Eqn 8, precomputing $(\mathbf{X}^\intercal \mathbf{W} \mathbf{y})$ and $(\mathbf{y}^\intercal \mathbf{W} \mathbf{y})$ further enables $\mathcal{O}(p)$ calculation of the loss after obtaining the optimal coefficients for the subset of basis functions, $\hat{\mathbf{b}}_A$.

$$\mathcal{L}(A) = SS_{\text{res}} = (\mathbf{y}^\intercal \mathbf{W} \mathbf{y}) - \hat{\mathbf{b}}_A (\mathbf{X}^\intercal \mathbf{W} \mathbf{y})_{AA} \tag{8}$$

At no point is the $\mathbf{X}$ matrix explicitly stored—reducing memory needs, which is critical for a distributed implementation where each process would otherwise need to store it. Since we freeze the radial parameters, this accuracy heuristic will tend to overestimate the loss. For our pruning case studies, we use the training data set and thus calculate training losses. However, it may be beneficial to use a separate validation set instead.

## Cost Heuristic

The cost objective function also uses a heuristic approach. Instead of measuring the runtime of a particular pruned MTP—which may be noisy and hardware dependent—we estimate the number of floating point operations (FLOPs) to evaluate a single neighborhood with Eqn. 9. We estimate the asymptotic cost, ignoring constant contributions. This particular formulation is based on the CPU variant of our Kokkos-based GPU implementation,[6] which has some speedups over MLIP-3, especially for smaller MTPs. The speedups will not be the same on GPU or with MLIP-3.

$$C(\nu_{\max}, \mu_{\max}, N_b, N_t) = n_{\text{neigh}}\big(24 + 4\nu_{\max} + 4\mu_{\max} N_Q + f(N_Q) + 39\, N_b\big) + 9\, N_t \qquad (9)$$

$\nu_{\max}$ is the maximum rank of any constituent moment tensors; $\mu_{\max}$ is the number of radial basis sets; $N_Q$ is the number of radial basis functions; $f(N_Q)$ is the cost to calculate the radial basis functions, which is $8N_Q + 14$ for the default radial basis set (`RBChebyshev`) from the MLIP packages. $n_{\text{neigh}}$ is the number of neighbors expected during inference, determining the relative importance of the number of root nodes, $N_b$, and $N_t$. For our case studies, we used the average value in the training set, although this can be adapted to better target production simulations of interest.

Practically, we precompute the necessary graph data using Alg. 1. At runtime, we can then compute $C(\nu_{\max}, \mu_{\max}, N_b, N_t)$ in $\mathcal{O}(|V| + |E|)$ with Alg. 2 which is based on breadth-

first search.

**Algorithm 1** Precompute Graph Properties

**Require:** MTP data
**Ensure:** Parent lists $\mathcal{P}$, maximum rank of the base potential $\nu_{\text{base}}$, maximum number of radial basis sets of the base potential $\mu_{\text{base}}$

1: Build parent lists $\mathcal{P}[k]$ from edges
2: Determine $\nu_{\text{base}}$
3: Determine $\mu_{\text{base}}$

# MTP Fitting Process

In both nickel and silicon–oxygen systems, the fitting results are highly dependent on the initialization; an MTP multiple levels larger could exhibit a worse training loss with a poor initialization than a smaller model with a strong initialization. This dependence was greater in Si–O.

The MLIP packages support random initialization and deterministic initialization. The deterministic initialization did not provide a better fit than the random initialization. For example, in Si-O at level 28, the deterministic initialization had a $3.3\times$ worse training loss than the potential we ultimately used.

Thus, we used random initialization. For each MTP, we trained 32 different trials for 450 BFGS steps. The choice of 450 steps was made because the last intermittent direct solution of the linear parameters in MLIP-3 is performed at 400 steps. Afterward, the 7 best seeds by training loss were then trained with no iteration limit, with the best result ultimately taken.

Default fitting parameters in MLIP-3 were used unless otherwise specified. The cutoff radius was 4 Å for Ni and 5.7 Å for Si-O, which also used a minimum distance of 0.8 Å. The Ni cutoff was retrieved from Zuo *et al.*,[7] and the Si-O cutoffs from Zongo *et al.*[8] The minimum distance for Ni was taken from the training data using MLIP-3's `mindist` functionality.

Notably, all MTPs generated in the case study used the default fitting mode (vibrations).

**Algorithm 2** Pruned MTP Cost Heuristic

**Require:** Set of retained indices $A$, parent lists $\mathcal{P}$, maximum base rank $\nu_{\text{base}}$, maximum base number of radial basis sets $\mu_{\text{base}}$
**Ensure:** Cost estimate $C$

Initialize counters to zero: number of basic nodes $N_b = 0$, number of edge pairs $N_t = 0$
Initialize boolean arrays $\nu[0 \ldots \nu_{\text{base}}] \leftarrow$ **false** and $\mu[0 \ldots \mu_{\text{base}}] \leftarrow$ **false**
Initialize queue $Q \leftarrow \emptyset$ and
Initialize visited$[k] \leftarrow$ **false** for all nodes $k$
**for all** index $i \in A$ **do**
Enqueue$(Q, i)$
visited$[i] \leftarrow$ **true**
**end for**
**while** $Q$ not empty **do**
$i \leftarrow$ Dequeue$(Q)$
**if** $i$ is basic **then**
$N_b \leftarrow N_b + 1$ ▷ Basic node retained
$\mu[$basis_of$(i)] \leftarrow$ **true** ▷ Flag this radial basis set
$\nu[$rank_of$(i)] \leftarrow$ **true** ▷ Flag this rank index
**else**
**for all** parents couples $p_1, p_2$ of $\mathcal{P}[i]$ **do**
$N_t \leftarrow N_t + 1$ ▷ Edge pair retained
**if** visited$[p_1]$ = **false then**
visited$[p_1] \leftarrow$ **true**
Enqueue$(Q, p_1)$
**end if**
**if** visited$[p_2]$ = **false then**
visited$[p_2] \leftarrow$ **true**
Enqueue$(Q, p_2)$
**end if**
**end for**
**end if**
**end while**
$\nu_{\max} \leftarrow$ number of true values in $\nu$
$\mu_{\max} \leftarrow$ number of true values in $\mu$
**return** $C(\nu_{\max}, \mu_{\max}, N_b, N_t)$

This fitting mode uses intensive energies and stresses. The potentials generated by Zongo *et al.* used structures mode, which scales the weight of the energy error by the inverse of the number of atoms in the configuration squared, and scales the weight of the force error by the inverse of the number of atoms in the configuration. Accordingly, the potential generated by Zongo *et al.* may favor a better fit on small configurations that are typically ordered structures. Zongo *et al.* also performed random initialization, although instead of choosing seeds by the training loss, they directly validated each seed on select physical properties.

## Multi-Objective Optimization

The list of indices, $A$, can be conveniently expressed as a binary vector, and uniform crossover can be applied. In each case study, the fitted level-28 MTP is used as the base potential for the multiobjective optimization using the parameters, and achieving the performance in Table 1. We presented the cost as the time spent on 64 cores in a single node (2 x AMD EPYC 7532) due to serial bottlenecks from the `pymoo` library.

Table 1: Parameters and performance. Default `pymoo` values are used unless otherwise specified.

| | **Ni** | | **SiO** | |
|---|---|---|---|---|
| **Parameters** | **NSGA-II** | **MOEA/D** | **NSGA-II** | **MOEA/D** |
| Cutoff Radius | 4 Å | | 5.7 Å | |
| Neighbor Count | 20.53 | | 46.02 | |
| Regularization ($\lambda$) | $10^{-2}$ | | $10^{-7}$ | |
| Mutation Operator | Random Single Bitflip | | | |
| Crossover | Uniform Crossover | | | |
| Population Size | 512 | 4096 | 512 | 4096 |
| Time taken on 64 cores | 3 days | 12 hours | 3 days | 12 hours |
| Generations | 92532 | 18414 | 89156 | 4781 |
| Evaluations | 47 Million | 75 Million | 45 Million | 19 Million |

We normalized the objective functions by dividing by the values of the base potential to better support MOEA/D, which depends on reference directions. Not doing so would heavily skew the directions against the cost objective function direction. MOEA/D could achieve

a higher evaluation rate due to the linear runtime of the serial `pymoo` code with population size. NSGA-II is quadratic with the population size. However, MOEA/D experienced issues with convergence for low-cost individuals, possibly due to our simplistic normalization.

# Silicon Physical Property Calculation Details

The lattice parameters were obtained by performing energy minimization of the crystal structures of silicon and $\alpha$-quartz.

For disordered systems, separate molecular dynamics simulations were carried out using each potential. In the case of liquid silicon, a system of 512 atoms was heated to 3000 K at a rate of 50 K/ps. The configuration was equilibrated at 3000 K for 30 ps, and the structural data was averaged over the last 10 ps of the simulation. To test the potential against amorphous silicon, we used the same heating approach. The liquid system was equilibrated at 2500 K and then cooled to 300 K at a rate of 10 K/ps. The configuration was subsequently relaxed in the NPT ensemble for 100,000 steps, and the structural data was averaged over the last 10 ps.

For liquid silica, the simulation started from a system containing 648 atoms. The structure was melted and pre-equilibrated using the level-22 MTP from Zongo *et al.*,[8] after which each potential was employed to equilibrate the system at 3000 K for 100 ps. Again, the structural data was averaged over the last 10 ps of the simulation.

# References


(1) Shapeev, A. V. Moment tensor potentials: A class of systematically improvable interatomic potentials. *Multiscale Modeling & Simulation* **2016**, *14*, 1153–1173.

(2) Wang, J.; Liu, P.; Zhu, H.; Liu, M.; Ma, H.; Chen, Y.; Sun, Y.; Chen, X.-Q. Efficient

moment tensor machine-learning interatomic potential for accurate description of defects in Ni-Al Alloys. *Physical Review Materials* **2025**, *9*, 053805.

(3) Novikov, I. S.; Gubaev, K.; Podryabinkin, E. V.; Shapeev, A. V. The MLIP package: moment tensor potentials with MPI and active learning. *Machine Learning: Science and Technology* **2020**, *2*, 025002.

(4) Podryabinkin, E.; Garifullin, K.; Shapeev, A.; Novikov, I. MLIP-3: Active learning on atomic environments with moment tensor potentials. *The Journal of Chemical Physics* **2023**, *159*.

(5) Thompson, A. P.; Swiler, L. P.; Trott, C. R.; Foiles, S. M.; Tucker, G. J. Spectral neighbor analysis method for automated generation of quantum-accurate interatomic potentials. *Journal of Computational Physics* **2015**, *285*, 316–330.

(6) Meng, Z.; Zongo, K.; Torres, E.; Maxwell, C.; Grant, R. E.; BÃŠland, L. K. A Kokkos-Accelerated Moment Tensor Potential Implementation for LAMMPS. *arXiv preprint arXiv:2510.00193* **2025**,

(7) Zuo, Y.; Chen, C.; Li, X.; Deng, Z.; Chen, Y.; Behler, J.; Csányi, G.; Shapeev, A. V.; Thompson, A. P.; Wood, M. A.; others Performance and cost assessment of machine learning interatomic potentials. *The Journal of Physical Chemistry A* **2020**, *124*, 731–745.

(8) Zongo, K.; Sun, H.; Ouellet-Plamondon, C.; Béland, L. K. A unified moment tensor potential for silicon, oxygen, and silica. *npj Computational Materials* **2024**, *10*, 218.
